# Supplementary material for: Assessment of error variation in high-fidelity two-qubit gates in silicon
Source: arXiv:2303.04090 ancillary file (2024-03-15)
Supplement: Supplementary file 1 [file 2Q_fidelity_supp.pdf]

## CONTENTS

|                                                                                           |    |
|-------------------------------------------------------------------------------------------|----|
| Supplementary Discussion: Comparison with other high fidelity two spin systems in silicon | 2  |
| A. Influence of a synthetic or natural spin-orbit field                                   | 2  |
| B. Influence of Material Properties                                                       | 2  |
| C. Gate Influence                                                                         | 3  |
| Supplementary Discussion: Randomised benchmarking                                         | 3  |
| Supplementary Discussion: Implementation of fast Bayesian tomography                      | 4  |
| D. Experiment designs for FBT                                                             | 5  |
| E. Parity readout as input for FBT                                                        | 6  |
| F. Gauge optimisation of FBT final estimated results                                      | 6  |
| G. Extracting error bar for FBT estimated fidelity                                        | 7  |
| Supplementary Discussion: Implementation of gate set tomography.                          | 7  |
| Supplementary Discussion: Gate set tomography with parity readout                         | 8  |
| Supplementary Discussion: Generator infidelity and total error                            | 10 |
| References                                                                                | 11 |

## SUPPLEMENTARY DISCUSSION: COMPARISON WITH OTHER HIGH FIDELITY TWO SPIN SYSTEMS IN SILICON

Our results may be compared to earlier studies of two-qubit gates in SiGe dots and phosphorus donors in silicon, where the fidelity analysis was demonstrated using randomized benchmarking<sup>1-3</sup>, GST<sup>4,5</sup>, or state tomography<sup>6</sup>. While all results have discussions on the physical sources of the errors, they focus mostly on the fidelity numbers achieved in two-qubit gates. Comparing the information in these works with our tomographies and previous knowledge about the physical properties of noise, we attempt to draw conclusions on the comparison between physical sources of errors in other material platforms as well.

Our combination of different tomographic methods allows for in-depth analysis of the physics of the errors. Firstly, we point out that combining the information from different sources allows for building a more complete microscopic picture of the qubits. The most immediate benefit of running tomographic analyses is that the full process matrix (with pyGSTi package<sup>7</sup>), can be used to extract the error channels which can be divided between stochastic and Hamiltonian error types. Hamiltonian errors in effect are all the errors that are in the same in every instance of the gate, irrespective of when in the circuit or lab time they are applied. Therefore, calibration errors, such as constant under/over rotation or cross talk between the qubits will appear as Hamiltonian error. Effectively everything else such as contextual shifts in the circuit time, or system shifts in the lab time, will appear as stochastic errors in most used GST schemes. Looking at the error generator channels can be very informative, though ultimately the physics must be interpreted by the user based on the knowledge of the underlying qubit system and the experimental setup.

As discussed in the main text, the non-Markovian errors (lab, and circuit time drifts) can be found in our spin qubits. Additional interesting aspect is provided by FBT, which through Bayesian inference follows the system parameters, instead of trying to fit the whole dataset at once<sup>7-9</sup>. Hence FBT shifts its Hamiltonian errors with the shifts in the lab time, though enough measurement statistic is needed for the FBT to capture changes in the system. In our main text we also utilize from the ability to perform FBT on circuits which are different total length, revealing the shift in the circuit time i.e. the contextual noise.

As mentioned earlier, some of the results earlier have significant similarities to our system. However, to achieve a meaningful comparison between platforms, we focus on Loss-DiVincenzo (single spin) qubit implementations achieved in dots with exchange control gates<sup>3,5</sup>. We note that Ref.<sup>2</sup> did not explicitly use exchange pulses, but other results achieved in the group do use pulsed exchange<sup>10,11</sup>. Interestingly, some of the error sources we observe can likely be observed in Refs.<sup>2-5</sup> as well. For instance, the contextual noise arising from the Larmor drift due to the microwave power is observed both in SiMOS and SiGe systems before<sup>12-14</sup>. However, when comparing these platforms, one should consider important physical differences between the SiMOS and SiGe platforms when extrapolating the possible physical error sources from our data in those systems.

### A. Influence of a synthetic or natural spin-orbit field

The spin-orbit interaction in a device is a result of natural relativistic effects in the material, but can also be artificially created through the use of a micro-magnet by applying a large magnetic field gradient, as demonstrated in<sup>2,3,5</sup>. In SiMOS devices, the variation of SiO<sub>2</sub> layer surface results in a natural varying Dresselhaus spin-orbit interaction<sup>15</sup> resulting in natural Zeeman energy differences between qubits. The ability to address single qubits to perform single qubit gates is necessary, meaning the Larmor frequencies should be sufficiently different if using electron spin resonance, otherwise gate defined gates should be implemented. Using a synthetic spin-orbit interaction, single qubit gates are defined by an oscillatory voltage on the top gate, moving the qubit within the magnetic field gradient to exhibit the electron to an oscillatory field called electric dipole spin resonance. As a result, this method of single qubit control has typically resulted in larger Rabi frequencies. Another advantage of using a micro-magnet is that you can tune the spin-orbit interaction, giving the ability to tune the Zeeman energy differences between qubits. However, a micro-magnet amplifies charge noise because it can couple to two-level fluctuators in the oxide. The micro-magnet spans a large area of the device, necessary to provide the magnetic field gradient across the qubit sites, resulting in the charge noise coupled to micro-magnet in turn influencing to multiple dot sites, as discussed in Ref.<sup>16</sup>.

### B. Influence of Material Properties

There also exist fundamental differences in the material stack of Si/SiGe and Si/SiO<sub>2</sub> devices. As the names suggest, one of the key differences lie in the material of the layer between the silicon channel and the metal gates, with SiGe being the interface material in previous studies<sup>2,3,5</sup>, and SiO<sub>2</sub> being the interface material in our case.

The  $\text{SiO}_2$  interface is formed by oxidising the surface layer of silicon at high temperatures, forming an amorphous layer above the bulk silicon, before the metal gate layers are deposited. Due to its intrinsically amorphous nature, this oxidation leads to a rough  $\text{SiO}_2$  interface, which alters the wavefunction of the electrons trapped in the silicon layer below the metal gates<sup>15</sup>.

This leads to some randomness in the several relevant qubit parameters, such as the formation of the dots (size, position, ellipticity), the interface-induced spin-orbit effect and the valley splitting<sup>15</sup>. This variability can be mitigated by, for instance, choosing the direction of the external magnetic field to minimize spin-orbit effects<sup>17</sup> or by encoding qubits in the valence state of multielectron quantum dots<sup>18</sup>. There also exists bounds to the impact of disorder on these parameters, which has been well studied and understood<sup>15</sup>. Another effect of the amorphous oxide layer is that it is also a source of two-level fluctuators which can exist close to where the qubits are formed (approximately 2 nm below the interface and into the silicon). These two-level fluctuators couple to the qubits as a form of charge noise, contributing towards the dominant source of noise for our qubits.

On the other hand, the Si/SiGe interface layer has two forms of disorder. First is the alloy disorder itself, which is natural to the fact that in an alloy at the atomic level the atoms of Ge are randomly distributed and therefore the exact atomic profile to which each quantum dot is exposed is slightly different and inhomogeneous. This effect gets amplified if the Ge atoms diffuse into the silicon well due to any high temperature processes in the fabrication.

The second form of interface disorder is associated with the angle of growth of the epitaxial layers with respect to the (001) lattice direction. Often, an intentional miscut angle is applied to reduce the stress in fabricating the Si/SiGe heterostructure and minimise the formation of defects, such as dislocations. This angle, however small, introduces steps to the Si/SiGe interface as a function of the in-plane position. Even for a very small miscut angle (which might not even be intentional) the density of interface steps is already comparable to the interdot distances, creating a high probability of a quantum dot forming at the edge of such a step.

In both cases, this disorder in the interface layer leads to several physical impacts on the qubits themselves. One of the physical sources of error is the hyperfine coupling to neighbouring isotopes that act as individual two-level systems which will lead to jumps in the Larmor frequency of the qubit whenever there is a nuclear spin flip in these isotopes. In the case of Si/ $\text{SiO}_2$  devices, this would be caused by the residual  $^{29}\text{Si}$ , while in the case of Si/SiGe devices, the  $^{73}\text{Ge}$  atoms in the interface layer also contribute to the effect, besides the  $^{29}\text{Si}$ .

In addition, it is also known that Germanium enhances spin-orbit coupling<sup>19,20</sup> and the  $^{73}\text{Ge}$  in the interface can couple to the electrons in the silicon and lead to a reduction in the coherence times of the electrons in Si<sup>21</sup>. Finally, the alloy disorder and interface steps are known to reduce valley splitting significantly<sup>22</sup>. The same is true for the roughness of the Si/ $\text{SiO}_2$  interface<sup>15</sup>, but the consistency of the valley splitting for Si/SiGe has been more challenging. Recent progress has been made in fabrication to significantly alleviate this issue<sup>23</sup>.

### C. Gate Influence

In order to form quantum dots in Si quantum well in Si/SiGe, metal gates are fabricated on top of SiGe spacer which is about 40 nm in thickness. On the other hand, for Si MOS quantum dots, metal gates are deposited on top of 8 nm high-quality  $\text{SiO}_2$  grown above silicon. The larger gate-to-dot distance in SiGe leads to a bigger dot size and hence larger lateral spread of electronic wavefunction. This larger dot size in SiGe has two sides to it: on one hand, the hyperfine coupling of single  $^{29}\text{Si}$  is lower on average leading to lower magnitude jumps for each  $^{29}\text{Si}$  atom that resides within the wavefunction of the dot. On the other hand, the more  $^{29}\text{Si}$  atoms lead to higher number of these small jumps and weaker nuclear freezing<sup>24</sup>.

Additionally, the larger distance between the silicon dot site and the gate controlling the exchange coupling, the lower is the level of controllability on the exchange with the gate. Hence in general, we would expect the level of controllability to be higher in SiMOS, though we note that the geometry used in SiGe in Ref.<sup>3</sup> had similar levels of exchange controllability compared to the ones in this paper. Higher controllability allows larger on-off ratios but subjects the two-qubit gate to voltage noise from the exchange gate during the operation. The voltage noise on the top gate is circumstantial though and our fidelity is not limited by this noise.

Lastly, the larger distance from the gate and  $\text{SiO}_2$  in SiGe reduces valley splitting<sup>23,25</sup>. Even though having difficulties from the low valley splitting, one major benefit of having the dots further away from the oxide is that they are less susceptible to the noise arising from the two level fluctuators in the amorphous  $\text{SiO}_2$ .

## SUPPLEMENTARY DISCUSSION: RANDOMISED BENCHMARKING

Interleaved randomised benchmarking (IRB) is commonly adopted in the literature for gate validation and is a relatively simple way of estimating the fidelity of a given gate. Two-qubit IRB is based on constructing all of the

11,520 Clifford gates from the primitive gates, which in our case are the single qubit gates  $X_1^{\pi/2}$ ,  $X_2^{\pi/2}$ ,  $Z_1^{\pi/2}$ ,  $Z_2^{\pi/2}$  and a two qubit gate, CZ or DCZ, depending on the experiment. Our implementations of the X gates are based on squarely pulsed microwave pulses that are timed to perform a  $\frac{\pi}{2}$  gate. Z gates are virtual and consist only of shifting the phase of all the subsequent pulses for that gate by  $\frac{\pi}{2}$ . The CZ gate is based on a square ramp of the exchange, on and off, to accumulate a phase difference of  $\pi$  between the qubits based on the state of the other. In a decoupled, two-qubit DCZ gate, the exchange pulse is split in half, with  $X^\pi$  pulses applied on both qubits in the middle of the pulse.

To run the randomised benchmarking, we generate a number (200 or 500) of randomised Clifford sequences of different lengths. This generation is done offline, split into smaller pieces and sent to the Field Programmable Gate Array (FPGA) that runs the experiment. Because of the memory constraints in the FPGA, we had to compile the sequences in a more memory efficient way, shown schematically in Figs. 1a and b. This is slightly different from the original randomised benchmarking protocol in terms of sequence lengths, but with enough randomisations this converges to the same sequence fidelity.

We fit the sequence fidelity as a function of the sequence length  $L$  to the function

$$f(L) = Ap_g^{L^n}, \quad (1)$$

where  $n$  and  $A$  are free parameters, though  $A$  is the same for both interleaved and reference sequences since it relates to visibility and  $p_g$  is the decay rate of the gate. In most common IRB analyses, the exponent  $n$  is fixed to one. However, using a super-exponentiated version allows us to better take care of the low frequency noise present in the system<sup>26</sup>, which will manifest as the exponent  $n > 1$ . For completeness, in table I, we show actual fidelities extracted using both methods of fitting for all runs and note that they do not differ from each other significantly. From the decay rates, we get the sequence fidelity by  $f_g = \frac{1}{4} + \frac{3}{4}d_g$  and  $d_{\text{int}} = p_{\text{int}}/p_{\text{ref}}$ , and  $d_{\text{ref}} = p_{\text{ref}}$ . One can also note that additional exponents in the super-exponential fit, for device A the value of  $n$  is around unity or just below. On the other hand for devices B and C,  $n$  averages at around 1.2, indicating an echoing effect taking place during the measurement due to the decoupling pulses included to the DCZ gate.

**Supplementary Table I:** Fidelities and fitting parameters of the interleaved randomised benchmarking, also shown in extended table III in the main text.

| Run                        | Clifford(%) (super-exp) | $n$ (super-exp) | CZ/DCZ(%) (super-exp) | $n$ (super-exp) | Clifford(%) (exp) | CZ/DCZ(%) (exp) |
|----------------------------|-------------------------|-----------------|-----------------------|-----------------|-------------------|-----------------|
| IRB <sub>1</sub> <b>A</b>  | 90.78 ± 0.10            | 1.020 ± 0.021   | 98.43 ± 0.22          | 0.893 ± 0.016   | 91.03 ± 0.11      | 98.57 ± 0.29    |
| IRB <sub>2</sub> <b>A</b>  | 90.71 ± 0.06            | 0.937 ± 0.014   | 98.41 ± 0.13          | 0.884 ± 0.013   | 91.26 ± 0.11      | 98.61 ± 0.31    |
| mean,std <b>A</b>          | 90.75, 0.05             |                 | 98.42, 0.01           | -               |                   |                 |
| IRB <sub>3</sub> <b>B</b>  | 86.95 ± 0.19            | 1.078 ± 0.029   | 99.00 ± 0.28          | 1.121 ± 0.016   | 86.36 ± 0.18      | 98.90 ± 0.35    |
| IRB <sub>4</sub> <b>B</b>  | 89.65 ± 0.06            | 1.143 ± 0.013   | 99.39 ± 0.11          | 1.133 ± 0.011   | 89.21 ± 0.13      | 99.34 ± 0.26    |
| IRB <sub>5</sub> <b>B</b>  | 85.06 ± 0.10            | 1.116 ± 0.014   | 99.33 ± 0.20          | 1.184 ± 0.017   | 84.12 ± 0.14      | 99.22 ± 0.36    |
| IRB <sub>6</sub> <b>B</b>  | 84.93 ± 0.09            | 1.103 ± 0.013   | 100.01 ± 0.17         | 1.196 ± 0.014   | 83.91 ± 0.12      | 99.95 ± 0.34    |
| IRB <sub>7</sub> <b>B</b>  | 86.13 ± 0.07            | 1.039 ± 0.010   | 99.32 ± 0.14          | 1.095 ± 0.010   | 85.54 ± 0.07      | 99.23 ± 0.18    |
| IRB <sub>8</sub> <b>B</b>  | 87.52 ± 0.07            | 1.133 ± 0.013   | 99.28 ± 0.14          | 1.181 ± 0.012   | 86.84 ± 0.14      | 99.19 ± 0.35    |
| IRB <sub>9</sub> <b>B</b>  | 87.29 ± 0.08            | 1.133 ± 0.014   | 99.20 ± 0.15          | 1.156 ± 0.013   | 86.57 ± 0.15      | 99.12 ± 0.32    |
| IRB <sub>10</sub> <b>B</b> | 86.90 ± 0.11            | 1.316 ± 0.029   | 99.68 ± 0.26          | 1.229 ± 0.029   | 85.67 ± 0.37      | 99.67 ± 0.68    |
| IRB <sub>11</sub> <b>B</b> | 87.19 ± 0.07            | 1.226 ± 0.014   | 99.14 ± 0.12          | 1.197 ± 0.011   | 86.11 ± 0.24      | 99.05 ± 0.46    |
| mean,std <b>B</b>          | 86.85, 1.41             |                 | 99.37, 0.3            | -               |                   |                 |
| IRB <sub>12</sub> <b>C</b> | 89.69 ± 0.11            | 1.454 ± 0.038   | 99.81 ± 0.29          | 1.393 ± 0.041   | 86.46 ± 0.47      | 99.70 ± 0.90    |
| IRB <sub>13</sub> <b>C</b> | 88.02 ± 0.13            | 1.863 ± 0.038   | 99.51 ± 0.28          | 1.866 ± 0.072   | 83.09 ± 0.79      | 99.24 ± 1.65    |
| IRB <sub>14</sub> <b>C</b> | 90.52 ± 0.09            | 1.210 ± 0.028   | 99.70 ± 0.23          | 1.249 ± 0.032   | 89.97 ± 0.24      | 99.69 ± 0.53    |
| IRB <sub>15</sub> <b>C</b> | 89.08 ± 0.10            | 1.049 ± 0.019   | 100.02 ± 0.24         | 1.001 ± 0.022   | 89.02 ± 0.13      | 100.04 ± 0.27   |
| mean,std <b>C</b>          | 89.33, 1.05             |                 | 99.76, 0.20           | -               |                   |                 |

## SUPPLEMENTARY DISCUSSION: IMPLEMENTATION OF FAST BAYESIAN TOMOGRAPHY

Based on previous work<sup>8</sup>, we have done several improvements to the FBT protocol to make it more robust and efficient for the analysis in this work. In this supplementary section, we explain how the experimental data for FBT is taken. Then we briefly explain the differences in this analysis method compared to the earlier work. Due to the heaviness of the analysis, we initially focused performing FBT on few particular IRB runs, especially the ones where we got the nonphysical value of above 100% fidelity. We note that this might cause some fidelity biasing. On the other hand, this offset by the lower Clifford fidelities in those runs, (partially the reason the interleaved sequence

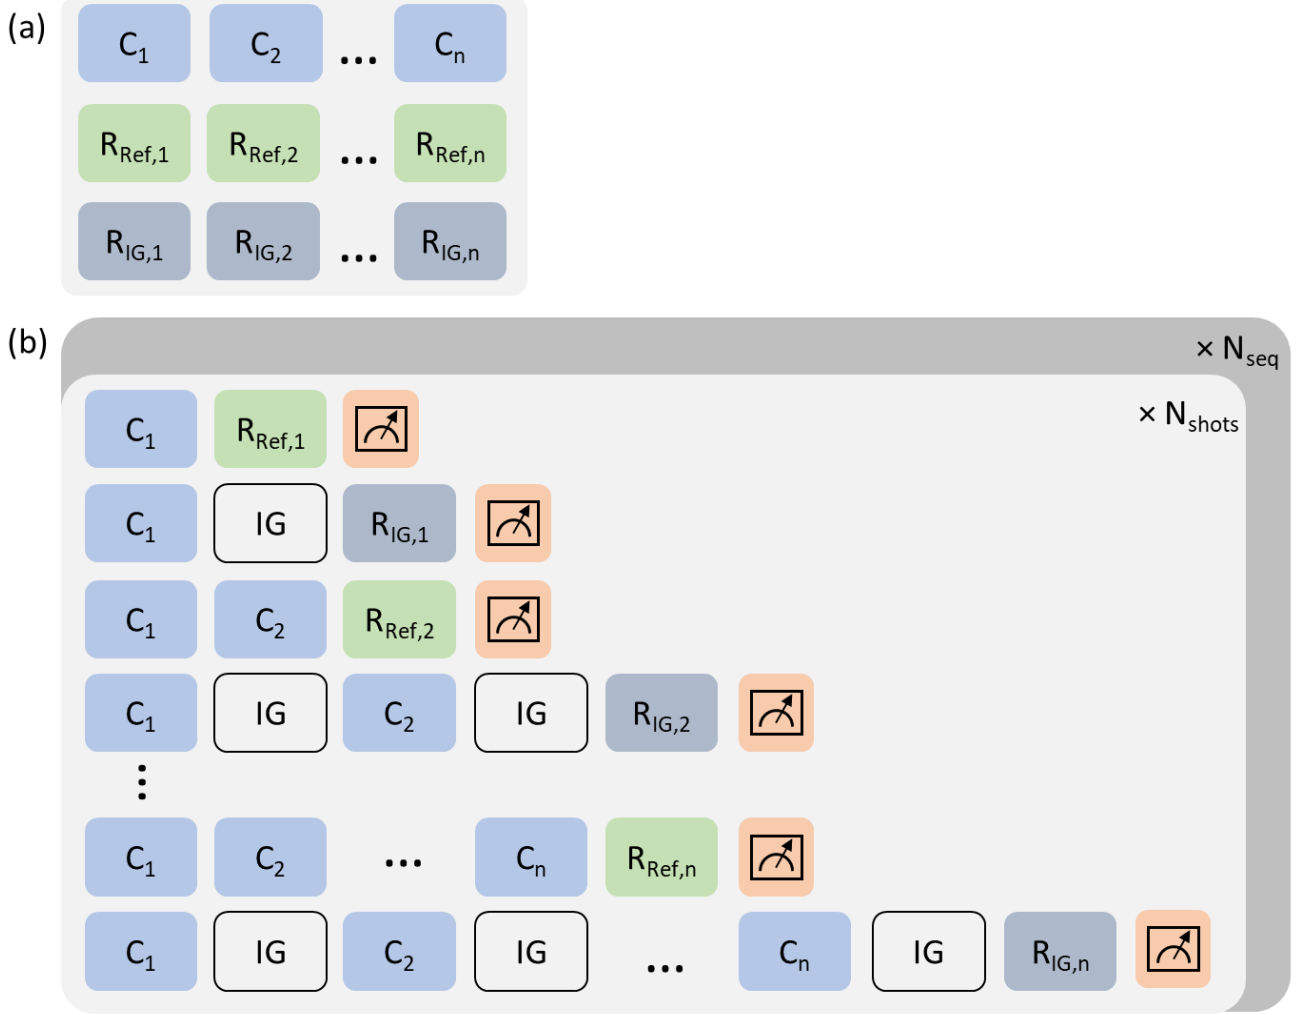

**Supplementary Figure 1: Schematic principle of randomised benchmarking principles.** **a** Input to the FPGA running the experiment for a single randomisation. Input is a set of randomly generated Clifford gates. Also we send a set of recovery gates for reference and interleaved sequences, for a sequence of length  $n$ . **b** The set of constructed measurement sequences from the input by the FPGA.

might have higher fidelity than the corresponding reference sequence). FBT will consider the CZ/DCZ gates that are included in the Clifford devices (1.5 in an average Clifford gate).

#### D. Experiment designs for FBT

From early characterisation, we have noticed non-Markovian behaviour of the gates in our system. As shown in Extended Figure 3 from the main text, we found that the gate behaves differently in sequences with different lengths and the gate performance can drift slowly due to sub-Hertz noise. This indicates that the way we run the experiments does matter when non-Markovian noise is present. The process tomography methods, including FBT and GST, are all based on the Markovian assumption. It would be helpful for improving the accuracy of the estimation if the experiments can be designed so that the inconsistency of a gate processed from sequence to sequence can be minimised.

Our experimental platform (Quantum Machine OPX) allows us to compile the gate sequences in real-time, which unlocks extra freedom for experimental design. The more data we provide to the QCVV protocols, the better error bars we can get from them. The experiment data acquisition time, the worst example being IRB, can take up to twelve

hours, which requires control electronics to loop over a large amount of sampling sequences and repeat each sequence for hundreds of shots. During these hours-long experiments, even with the implemented feedback protocols, gate performances can still slowly drift over time (See Fig.4). We program the field programmable gate array (FPGA) to loop all sequences for the innermost loop and then run to the next repeat of all of the sequence loops. This rasterised manner allows the slow drift noise to impact evenly over all sequence results, thus, the non-Markovianity of the data will be suppressed at the inter-sequence level. By doing this, we are not eliminating the slow drift from the physical system, but the inter-sequence inconsistency can be averaged out, shot-wise.

To investigate how gate performance changes with different sequence lengths, we perform a sequence length dependency experiment. Each experiment generates 5000 random sequences with same length, with each sequence repeated for 100 shots. Since one experiment will consume around 20 minutes, to minimise the impact from slow drifting or sub-Hertz noise, we run sequences in a rasterised manner as mentioned above. Though FBT is not characterising the non-Markovian dynamics, which requires more complicated techniques like process tensor tomography, the length dependency results display a significant inconsistency of the gate performance for different sequence lengths and can indicate which channel parameters have most inconsistency.

Interleaved randomised benchmarking, though not designed for FBT, has an informational completeness suitable for FBT analysis. A typical IRB experiment can take hours to finish and the inter-sequence consistency of the data can be harmed due to the slow drift of the system. To fight against the slow drift issue and give a good fit for IRB, the rasterized loop is preferred, though not always a possible choice. However, putting tens of thousands of sequences all together into a single loop will overload the FPGA programming memory. To resolve this, we divide the sequence set into batches and sending them to the FPGA memory individually. Each batch of sequences, running in a rasterized manner, contains sequences with Clifford lengths ranging from minimum to maximum length from the parent set. Each batch of IRB takes around 40 seconds and we have 200 to 500 batches in total. Based on earlier characterisation and feedback data, we believe that the slow drift is relatively static within that time window and from batch to batch the slow drift is continuous. Generally, the intermediate FBT results are meaningless and we only take the last update as the most trusted estimation. We bootstrap the initial priors by injecting gate fidelities estimated from a recent FBT-IRB run, then, by the time we receive the first batch of IRB results, the model is already standing on the best guess of the fidelities and the new incoming data will update the model based on that prior. Similarly, the later incoming batches of IRB results can be bootstrapped by the posterior of the previous batch update. Thus, estimated results from FBT for each batch can be approximately treated as a pseudo-transient state of its corresponding lab time. Though the best-guessed fidelity bootstrapping is not accurately addressing the transient fidelity number, it provides a relatively reliable start point for tracking the fidelity drifts for the gate set. There are two major limitations of this performance-tracking method. First, in a limited time window, it is hard to guarantee the informational completeness of the data we have obtained. Secondly, the covariance of the multi-variate Gaussian statistic keeps diminishing as we update the model with more data under the Markovian assumption, which slows down the speed of convergence of the model under a slow-drifting scenario.

### E. Parity readout as input for FBT

In this paper, we are measuring the pair of qubits in a parity basis. Each shot of experiment is offering either blockaded/unblockaded binary information by tunnelling the electron from one dot to another. For example, a even parity will output a blockaded result as the SET keeps silent during the readout time window. The parity outcomes are degenerate, for example, even parity can be either  $\uparrow\uparrow$  or  $\downarrow\downarrow$  states. As such, the measurement super vector for the FBT model can be constructed as:

$$\begin{aligned} E_{\text{odd}} &= |\uparrow\downarrow\rangle\langle\uparrow\downarrow| + |\downarrow\uparrow\rangle\langle\downarrow\uparrow| \\ E_{\text{even}} &= |\uparrow\uparrow\rangle\langle\uparrow\uparrow| + |\downarrow\downarrow\rangle\langle\downarrow\downarrow| = G_{X_2^{\pi/2}} G_{X_2^{\pi/2}} [E_{\text{odd}}]. \end{aligned} \quad (2)$$

By updating the primitive parity readout results to FBT directly, we avoid linear transformation from parity basis to qubit basis, which can not guarantee the completely positive trace-preservation (CPTP) of the reconstructed states.

### F. Gauge optimisation of FBT final estimated results

The outputs from the FBT experiments are essentially multi-variable Gaussian statistics of the channel parameters which are trying to minimise the distance between the experiment outcome and model inference. However, the representation of the best estimated model is not unique, an outcome that is also known as gauge ambiguity. By gauge-transforming the estimated gate set together with SPAM channels, it does not change the observable probabilities that

the model infers. The previous work<sup>8</sup> avoids this gauge ambiguity by assuming preparations are always perfect, so that the model will have a fixed gauge. For the FBT analysis in this work, we are no longer holding this assumption and initialising the model with preparation and measurement channel. In this work, we have implemented gauge optimisation for FBT based on optimising the weighted Frobenius distance between the estimated model and ideal model<sup>7</sup>.

### G. Extracting error bar for FBT estimated fidelity

As shown in Algorithm 1, the error bar of FBT estimated gate fidelities are extracted by Gaussian sampling of the Bayesian statistics, including the estimated gate error channel mean and its covariance matrix. In this work, every fidelity statistic is obtained by resampling the channel 100 times.

---

#### Algorithm 1: Error bar for FBT estimated fidelity

---

**Input:**  $\bar{\Lambda}$ : Estimated noise channel mean  
**Input:**  $\Gamma_{\Lambda}$ : Estimated covariance matrix for the channel  
 $\Lambda \sim \mathcal{N}(\bar{\Lambda}, \Gamma_{\Lambda})$   
**for**  $i = 0$  **to**  $N_{sample}$  **do**  
    Gaussian sample a noise process matrix  $\mathcal{X}$   
     $Fidelity(\mathcal{X}) = 1 - \frac{d^2 - Tr(\mathcal{X})}{d^2 + d}$   
    where  $d = dimension\{\mathcal{X}\}$   
    Save  $f_{\mathcal{X}}$  to  $P(f)$   
**end**  
 $\bar{f}' \leftarrow mean(P(f))$   
 $\sigma'_f \leftarrow cov(P(f))$   
**Output:**  $(\bar{f}', \sigma'_f)$

---

**Supplementary Table II:** Fidelities extracted from the FBTs from several IRB runs for all devices (see also the Extended Table III). Here, we show the average fidelity over the whole run (error bars  $2\sigma$  variation) and together with the best and the worst gates in the experiment together with the error of the FBT estimation at that point.

| Run          | CZ/DCZ(%)        | best             | worst            | $X_1^{\pi/2}$ (%) | best (%)         | worst            | $X_2^{\pi/2}$ (%) | best             | worst            |
|--------------|------------------|------------------|------------------|-------------------|------------------|------------------|-------------------|------------------|------------------|
| FBT <b>A</b> | $98.35 \pm 0.54$ | $98.64 \pm 0.25$ | $98.15 \pm 0.2$  | $98.41 \pm 0.89$  | $99.07 \pm 0.53$ | $98.03 \pm 0.30$ | $99.09 \pm 0.78$  | $99.55 \pm 0.25$ | $98.67 \pm 0.21$ |
| FBT <b>B</b> | $99.03 \pm 0.91$ | $99.65 \pm 0.51$ | $98.70 \pm 0.33$ | $95.92 \pm 0.78$  | $96.31 \pm 0.43$ | $95.18 \pm 0.88$ | $96.58 \pm 0.66$  | $96.89 \pm 0.48$ | $95.79 \pm 1.08$ |
| FBT <b>C</b> | $99.04 \pm 0.54$ | $99.43 \pm 0.27$ | $98.64 \pm 0.14$ | $97.00 \pm 1.16$  | $97.37 \pm 0.38$ | $95.96 \pm 0.65$ | $97.72 \pm 0.87$  | $98.47 \pm 0.65$ | $97.12 \pm 0.46$ |

### SUPPLEMENTARY DISCUSSION: IMPLEMENTATION OF GATE SET TOMOGRAPHY.

In this paper, we performed gate set tomography using the pyGSTi package<sup>7,27</sup>. The general workflow of the tomography analysis is outlined in Fig. 2(c) of the main text. Gate set tomography (GST) utilizes specially designed gate sequences to obtain high-precision information about the errors in our system. The first step in the construction of a GST experiment design is to generate an informationally complete set of preparation and measurement fiducial circuits and an amplificationally complete set of germs<sup>7</sup>. When combined, these form the set of gate sequences to be run.

We perform a novel variation of two-qubit GST<sup>4</sup> adapted to the unique properties of this system. Previous experiments leveraged simultaneous readout of both qubits individually, which is described by a four-outcome positive operator-valued measure (POVM)  $\{|00\rangle\langle 00|, |01\rangle\langle 01|, |10\rangle\langle 10|, |11\rangle\langle 11|\}$ . Our systems use a parity readout, described by a two-outcome POVM  $\{|00\rangle\langle 00| + |11\rangle\langle 11|, |10\rangle\langle 10| + |01\rangle\langle 01|\}$ . This requires only one change to the GST experiment design: definition of a new and slightly larger set of “measurement fiducial” circuits. Measurement fiducials, labeled  $\mathcal{F}_k$  in Fig. 2c, are short subcircuits used to probe an informationally complete set of different observables. The measurement fiducial construction used for this experiment is described in the Supplementary Discussion: Gate Set Tomography with parity readout, where we also compare our results to an emulated “standard GST” experiment on this device. The observed outcome frequencies for all GST circuits are fed into the GST analysis software package pyGSTi<sup>7</sup>, which returns estimates of the gate process matrices. The GST estimate of the DCZ gate is shown in Figs. 2d, 2e, 2f, and 2g in main text and in the Extended Tables IV(a) and IV(b) we quantify the errors in our

gates using two metrics, generator infidelity and total error<sup>4,28</sup>. In these tables we have additionally partitioned both metrics according to their support in order to distinguish errors that occur locally on a gate's target qubit from ones afflicting a spectator qubit (e.g., due to crosstalk, see the Supplementary Discussion: Gate Set Tomography with parity readout for more details).

In our experiments, we perform an X rotation gate via ESR pulsing from the microwave antenna (see Fig. 1(a) of the main text). Our Z rotation gates are performed virtually as a frame rotation in the FPGA. These two gates are then combined to perform Y rotations, where we first perform a frame rotation using the virtual Z gate and then perform an X rotation. The gate set used for the GST analysis of our system comprises the single-qubit  $X_1^{\pi/2}$ ,  $X_2^{\pi/2}$ ,  $Z_1^{\pi/2}$  and  $Z_2^{\pi/2}$  gates (which are the natural gates in our system), along with the two-qubit entangling CZ gate for device A or the DCZ gate for device B.

### Supplementary Discussion: Gate set tomography with parity readout

Analyzing our system using GST while utilizing native parity readout requires a few modifications to the design of our experiments and to the analysis workflow. While the pyGSTi software package provides built-in experimental designs for the gate sets investigated in this work, these assume access to bit-wise readout in the computational basis and the corresponding measurement fiducials are not informationally complete when using parity readout. As such, while it is straightforward to define a gate set model utilizing parity readout in pyGSTi, it is still necessary to construct new experimental designs that are informationally complete.

Our initial construction of the experimental designs for GST using parity readout leveraged the observation that, while we don't have access to computational basis readout, we can simulate computational basis readout for any given circuit by running that circuit six times, each time with a different short subcircuit appended to it. We call these additional subcircuits *projections*. By appropriately combining the parity readout statistics for each of these six projected circuits we can simulate what the output statistics of that circuit would have been using computational basis readout. The six projection sequences are:

1.  $\{\}$  — Do nothing.
2.  $X_\pi(Q_2)$  —  $\pi$  pulse on qubit 2.
3.  $\text{CNOT}(Q_1) + X_\pi(Q_2)$  — CNOT on qubit 1 followed by a  $\pi$  pulse on qubit 2.
4.  $\text{CNOT}(Q_1)$  — CNOT on qubit 1.
5.  $\text{CNOT}(Q_2) + X_\pi(Q_2)$  — CNOT on qubit 2 followed by a  $\pi$  pulse on qubit 2.
6.  $\text{CNOT}(Q_2)$  — CNOT on qubit 2.

Given these projections, the output statistics for computational basis readout can be simulated by taking linear combinations of the estimated outcome probabilities for parity readout,

$$\begin{aligned}
 p_{00} &= \frac{1}{4} (p_{e,1} + p_{e,4} + p_{e,6} - p_{e,2} - p_{e,3} - p_{e,5} + 1) \\
 p_{01} &= \frac{1}{4} (p_{e,2} + p_{e,3} + p_{e,6} - p_{e,1} - p_{e,4} - p_{e,5} + 1) \\
 p_{10} &= \frac{1}{4} (p_{e,2} + p_{e,4} + p_{e,5} - p_{e,1} - p_{e,3} - p_{e,6} + 1) \\
 p_{11} &= \frac{1}{4} (p_{e,1} + p_{e,3} + p_{e,5} - p_{e,2} - p_{e,4} - p_{e,6} + 1),
 \end{aligned} \tag{3}$$

where  $p_{e,i}$  denotes the estimated probability for even parity when measuring the  $i^{\text{th}}$  projection of a circuit. It follows that if we can use these projection sequences to simulate computational basis measurement using the native parity readout then we can also use these sequences to construct a set of measurement fiducials that is informationally complete with respect to the native parity readout. To do so, we simply took a set of measurement fiducials meant for computational basis readout and appended to each of them the six different projection sequences. This gives a set of measurement fiducials six times larger than the original measurement fiducial set it is constructed from, but which is guaranteed by construction to be informationally complete for the native parity readout.

This initial construction is massively over-complete (with over 60 fiducials), so as a final step, we utilized the fiducial selection infrastructure available in pyGSTi to identify a significantly smaller subset of 16 measurement fiducials from

among the initial construction that was informationally complete for the parity readout. GST analysis using the larger initial set of measurement fiducials is presented in the main text, as the larger data set allows for tighter error bars on our estimates. A natural question is whether the significant reduction in the size of the experiment design achieved by pruning the original construction meaningfully impacts our final estimates. To answer this we collected data for the full initial measurement fiducial construction rather than just the reduced set of 16.

Constructing GST estimates using the reduced set of measurement fiducials does not meaningfully change our final results compared to using the much larger initial construction. This can be seen in Table III where we compare the estimated entanglement infidelities for all three estimates on both devices A and B. For both sets of measurement fiducials the entanglement fidelities are consistently within error bars of each other across all of the gates in the gate set. This confirms that the estimates are largely consistent for both experiment designs, so there is little value in performing the significantly larger experiment.

In addition to comparing the estimated error parameters for the two experimental designs as we did in Table III, we can also assess the quality of the GST fits directly by looking to see how consistent the predictions of the estimated gate sets are with the datasets they were fit from. Figure 2 compares the per-sequence model-violation statistics for the GST fit estimated with respect to each of these sets of measurement fiducials. These model violation statistics are computed using log-likelihood ratio statistics, and from Wilks' theorem are expected to follow a  $\chi_n^2$  distribution, where  $n$  is the number of possible independent measurement outcomes for a sequence. Figure 2a presents histograms of the model-violation statistics for device A, while Figure 2b presents these results for device B. For both devices A and B we can see that the distribution of the per-sequence model violation statistics are essentially unchanged between fits based on the full initial fiducial construction and the more minimal set. This indicates that the quality of our fits were not meaningfully changed by fitting our GST estimates with respect to the significantly smaller data set. While actually performing the simulation of computational basis readout which motivated the construction of measurement fiducials for the native parity readout is generally not advisable (as will be demonstrated shortly), since the data required to do so was available we also produced a GST estimate using simulated computational basis readout. Figures 2c and 2d present the model violation statistics for devices A and B respectively. Compared to the fits performed with respect to the native parity readout, the estimates produced using simulations of computational readout show significant increases in the amount of per-sequence model violation. This phenomenon arises as a result of two key effects. First, taking linear combinations of estimated outcome probabilities as done in Equation 3 distorts the behavior of the log-likelihood ratio statistic, which leaves us unable to evaluate the quality of the resulting GST fits without a more sophisticated analysis.

Second, the estimation of the parity readout probabilities required for forming the requisite linear combinations requires augmenting a base circuit whose outcome probabilities we're interested in estimating with additional short projection sequences. These projection sequences introduce additional noise that is generally different for each projection and is not accounted for in Equation 3. Thus, while intellectually valuable for reasoning about experiment design construction, actually implementing simulations of computational basis readout is inadvisable for the purposes of device characterization.

**Supplementary Table III:** Gate entanglement infidelities from GST characterization of devices A and B for different variants of the experiment design. Note that Device A uses a CZ gate while Device B uses the dynamically-decoupled DCZ gate.

| Gate          | Device A    |             |            | Device B    |             |            |
|---------------|-------------|-------------|------------|-------------|-------------|------------|
|               | Min. Parity | Full Parity | Projection | Min. Parity | Full Parity | Projection |
| $X_1^{\pi/2}$ | 4.4(5)%     | 4.4(3)%     | 4.4(3)     | 2.9(4)%     | 2.6(3)%     | 2.5(2)%    |
| $X_2^{\pi/2}$ | 3.2(4)%     | 3.2(3)%     | 3.0(2)%    | 5.2(3)%     | 5.3(2)%     | 5.2(2)%    |
| $Z_1^{\pi/2}$ | 0.5(3)%     | 0.3(2)      | 0.1(2)%    | 0.6(3)%     | 0.4(2)%     | 0.3(2)%    |
| $Z_2^{\pi/2}$ | 0.5(3)%     | 0.4(2)%     | 0.01(20)%  | 0.4(3)%     | 0.4(2)%     | 0.2(2)%    |
| CZ            | 4.0(5)%     | 4.0(3)%     | 4.3(3)%    |             |             |            |
| DCZ           |             |             |            | 2.7(3)%     | 2.5(2)%     | 2.1(2)%    |

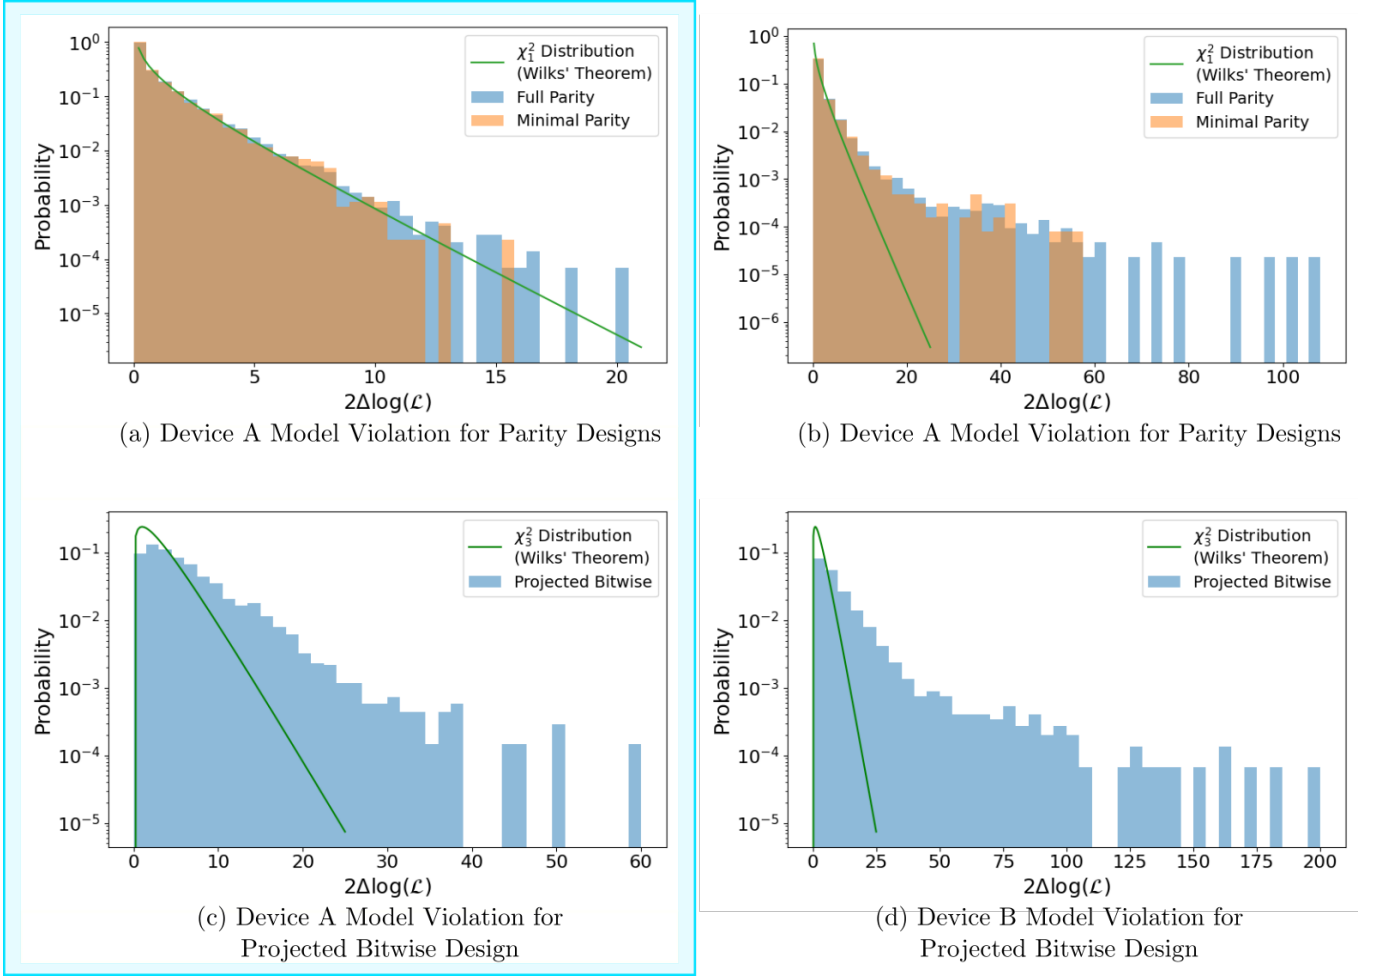

**Supplementary Figure 2:** Normalized per-circuit model violation histograms for native parity readout based designs (top row) and projected bitwise (i.e. simulated computational basis) readout based designs (bottom row) for Device A (left column) and Device B (right column). The solid green lines superposed on top indicate the expected  $\chi^2$  distribution of the per-sequence model violation under Wilks' theorem. The outlined panels for Device A highlight the undesired model violation introduced by the 6-fold projection scheme.

### Supplementary Discussion: Generator infidelity and total error

Extended Tables IV(a) and IV(b) showed the generator infidelities of the gates taking into account the cross talk etc. The generator infidelity,  $\hat{\epsilon}$ , and total error,  $\epsilon_{\text{tot}}$  are defined as

$$\hat{\epsilon} = \sum_i \epsilon_i + \sum_i \theta_i^2 \quad (4)$$

$$\epsilon_{\text{tot}} = \sum_i \epsilon_i + \sqrt{\sum_i \theta_i^2}, \quad (5)$$

where  $\{\epsilon_i\}$  and  $\{\theta_i\}$  are the rates of stochastic and Hamiltonian errors, respectively (see Fig. 3). To obtain single-qubit generator infidelities for each of the two qubits, we replace the sums in Equations 4 and 5 with sums over only error generators supported solely on that qubit. For more on generator infidelity, total error, and their connection to entanglement infidelity and diamond distance, see the supplementary material of Ref.<sup>4</sup>.

One feature that jumps out from Tables IV(a) and IV(b) is that the error budgets of the single qubit gates are dominated by crosstalk<sup>29</sup>. Take, for example, the  $X_1^{\pi/2}$  gate on Device B where we can see that, of the 2.7% total generator infidelity for this gate,  $\sim 85\%$  of that infidelity is attributable to unwanted dynamics local to the spectator

qubit. In fact, we only attribute  $\sim 4\%$  of the infidelity to noise directly on the target qubit (with the remaining error budget attributed to higher weight multi-qubit noise processes). The dominance of crosstalk effects in the error budget for the gates is consistent across the single-qubit X gates on both device A and B.

- 
- <sup>1</sup> Huang, W. *et al.* Fidelity benchmarks for two-qubit gates in silicon. *Nature* **569**, 532–536 (2019). URL <https://doi.org/10.1038/s41586-019-1197-0>.
  - <sup>2</sup> Noiri, A. *et al.* Fast universal quantum gate above the fault-tolerance threshold in silicon. *Nature* **601**, 338–342 (2022). URL <https://doi.org/10.1038/s41586-021-04182-y>.
  - <sup>3</sup> Mills, A. R. *et al.* Two-qubit silicon quantum processor with operation fidelity exceeding 99%. *Science Advances* **8**, eabn5130 (2022). URL <https://www.science.org/doi/abs/10.1126/sciadv.abn5130>. <https://www.science.org/doi/pdf/10.1126/sciadv.abn5130>.
  - <sup>4</sup> Mądzik, M. T. *et al.* Precision tomography of a three-qubit donor quantum processor in silicon. *Nature* **601**, 348–353 (2022). URL <https://doi.org/10.1038/s41586-021-04292-7>.
  - <sup>5</sup> Xue, X. *et al.* Quantum logic with spin qubits crossing the surface code threshold. *Nature* **601**, 343–347 (2022). URL <https://doi.org/10.1038/s41586-021-04273-w>.
  - <sup>6</sup> Weinstein, A. J. *et al.* Universal logic with encoded spin qubits in silicon. *Nature* **615**, 817–822 (2023). URL <https://doi.org/10.1038/s41586-023-05777-3>.
  - <sup>7</sup> Nielsen, E. *et al.* Gate Set Tomography. *Quantum* **5**, 557 (2021). URL <https://doi.org/10.22331/q-2021-10-05-557>.
  - <sup>8</sup> Evans, T. *et al.* Fast bayesian tomography of a two-qubit gate set in silicon. *Phys. Rev. Applied* **17**, 024068 (2022). URL <https://link.aps.org/doi/10.1103/PhysRevApplied.17.024068>.
  - <sup>9</sup> Su, R. Y. *et al.* Characterizing non-markovian quantum process by fast bayesian tomography (2023). 2307.12452.
  - <sup>10</sup> Takeda, K. *et al.* Quantum tomography of an entangled three-qubit state in silicon. *Nature Nanotechnology* **16**, 965–969 (2021). URL <https://doi.org/10.1038/s41565-021-00925-0>.
  - <sup>11</sup> Takeda, K., Noiri, A., Nakajima, T., Kobayashi, T. & Tarucha, S. Quantum error correction with silicon spin qubits. *Nature* **608**, 682–686 (2022). URL <https://doi.org/10.1038/s41586-022-04986-6>.
  - <sup>12</sup> Freer, S. *et al.* A single-atom quantum memory in silicon. *Quantum Science and Technology* **2**, 015009 (2017). URL <https://dx.doi.org/10.1088/2058-9565/aa63a4>.
  - <sup>13</sup> Takeda, K. *et al.* Optimized electrical control of a Si/SiGe spin qubit in the presence of an induced frequency shift. *npj Quantum Information* **4**, 54 (2018). URL <https://doi.org/10.1038/s41534-018-0105-z>.
  - <sup>14</sup> Undseth, B. *et al.* Hotter is easier: unexpected temperature dependence of spin qubit frequencies (2023). 2304.12984.
  - <sup>15</sup> Cifuentes, J. D. *et al.* Bounds to electron spin qubit variability for scalable cmos architectures (2023). 2303.14864.
  - <sup>16</sup> Yoneda, J. *et al.* Noise-correlation spectrum for a pair of spin qubits in silicon. *Nature Physics* **19**, 1793–1798 (2023).
  - <sup>17</sup> Tanttu, T. *et al.* Controlling spin-orbit interactions in silicon quantum dots using magnetic field direction. *Phys. Rev. X* **9**, 021028 (2019). URL <https://doi.org/10.1103/physrevx.9.021028>.
  - <sup>18</sup> Leon, R. *et al.* Coherent spin control of s-, p-, d- and f-electrons in a silicon quantum dot. *Nature Communications* **11**, 797 (2020). URL <https://doi.org/10.1038/s41467-019-14053-w>.
  - <sup>19</sup> Liu, L. Effects of spin-orbit coupling in si and ge. *Physical Review* **126**, 1317 (1962).
  - <sup>20</sup> Zhang, X. *et al.* Universal control of four singlet-triplet qubits. *arXiv preprint arXiv:2312.16101* (2023).
  - <sup>21</sup> Witzel, W. M., Rahman, R. & Carroll, M. S. Sige/si quantum dot electron spin decoherence dependence on <sup>73</sup> ge. *arXiv preprint arXiv:1110.4143* (2011).
  - <sup>22</sup> Losert, M. P. *et al.* Practical strategies for enhancing the valley splitting in si/sige quantum wells. *Phys. Rev. B* **108**, 125405 (2023). URL <https://link.aps.org/doi/10.1103/PhysRevB.108.125405>.
  - <sup>23</sup> Lodari, M. *et al.* Valley splitting in silicon from the interference pattern of quantum oscillations. *Phys. Rev. Lett.* **128**, 176603 (2022). URL <https://link.aps.org/doi/10.1103/PhysRevLett.128.176603>.
  - <sup>24</sup> Mądzik, M. T. *et al.* Controllable freezing of the nuclear spin bath in a single-atom spin qubit. *Science Advances* **6**, eaba3442 (2020). URL <https://www.science.org/doi/abs/10.1126/sciadv.aba3442>. <https://www.science.org/doi/pdf/10.1126/sciadv.aba3442>.
  - <sup>25</sup> Saraiva, A. L., Calderón, M. J., Hu, X., Das Sarma, S. & Koiller, B. Physical mechanisms of interface-mediated intervalley coupling in si. *Phys. Rev. B* **80**, 081305 (2009). URL <https://link.aps.org/doi/10.1103/PhysRevB.80.081305>.
  - <sup>26</sup> Fogarty, M. A. *et al.* Nonexponential fidelity decay in randomized benchmarking with low-frequency noise. *Phys. Rev. A* **92**, 022326 (2015). URL <https://link.aps.org/doi/10.1103/PhysRevA.92.022326>.
  - <sup>27</sup> Greenbaum, D. Introduction to quantum gate set tomography. *arXiv preprint arXiv:1509.02921* (2015).
  - <sup>28</sup> Blume-Kohout, R. *et al.* A taxonomy of small markovian errors. *PRX Quantum* **3**, 020335 (2022). URL <https://link.aps.org/doi/10.1103/PRXQuantum.3.020335>.
  - <sup>29</sup> Sarovar, M. *et al.* Detecting crosstalk errors in quantum information processors. *Quantum* **4**, 321 (2020). URL <https://doi.org/10.22331/q-2020-09-11-321>.
